# Supplementary material for: An Empirical Study on Robustness to Spurious Correlations using Pre-trained Language Models
Source: arXiv:2007.06778 source file (2020-08-11)
Supplement: Supplementary file 1 [file appendices.tex]

\section{Appendices}

Table~\ref{tab:pretrainedBert_more} and Table~\ref{tab:finalnli_more} show some experiment results on the three subsets of HANS.
Table~\ref{tab:pretrainedBert_more} shows the non-pretrained model and pretraind model results. And Table~\ref{tab:pretrainedBert_more} shows the model performance when adding the auxiliary datasets. 

\begin{table*}[ht]
\footnotesize{
  \begin{center}
  \tabcolsep 2pt
    \begin{tabular}{cccc} 
    \toprule
       Model   & \textbf{HANS-O(\%)}   & \textbf{HANS-C(\%)} & \textbf{HANS-S(\%)}     \\
      \midrule
      \multicolumn{1}{l}{\textbf{Non-pretrained Models}} \\
      \rbert  & 49.9(.04) & 49.3(0.1) & 50.3(0.4) \\ \hline \hline
      \multicolumn{1}{l}{\textbf{Pretrained Models}} \\
      %BERT$_{base}$(4 epochs) & MNLI-en & 84.5  & -  & - & - & 58.3  \\
      %\small{\citet{clark-etal-2019-dont}} &  & 84.2  &- & -& -& 62.4 \\
      \bert   & 75.8(4.9) & 59.1(4.8) & 52.7(1.2) \\
      \bertl  & 88.6(1.6) & 66.4(0.8) & 59.0(1.6) \\
      %Openwebtext-BERT  & 83.7/0.4 & 88 & 49 & & 68.2 \\ 
      \roberta & 88.5(2.0) & 70.0(2.3) & 63.9(1.4)  \\
      \robertal & 96.7(2.2) & 71.2(1.0) & 63.5(3.4) \\
      %mBERT$_{base}$ & MNLI-en & 82.7 & 76.3 &- &- & 65.0 \\
      %mBERT$_{base}$ & + translate & 58.0 &- &- &- &52.5 \\
      \bottomrule
    \end{tabular}
  \caption{\label{tab:pretrainedBert_more}Performance on HANS lexical overlap (HANS-O), HANS constituent (HANS-C) dataset, HANS subsequence (HANS-S) dataset when fine-tuning different BERTs: \rbert, \bert, \bertl, \roberta, and \robertal.  \rbert is \bert model with random initialization. For all the models, we do early stopping on the MNLI dev set and shows the means and standard deviations with 5 runs with different random seeds. The numbers in the bracket are the standard deviations of the 5 runs.}
  \end{center}
  }
\end{table*}

\begin{table*}[t]
\footnotesize{
 \begin{center}
\begin{tabular}{ccccc}
%\toprule
 Task Data - Aux Data & \textbf{HANS-O(\%)} & \textbf{HANS-C(\%)}  &  \textbf{HANS-S(\%)}\\ 
 %\cline{3-7}
 %\midrule
 %MNLI(other paper), - & &  &  &  & \\
 MNLI  -  & 75.8(4.9) & 59.1(4.8) & 52.7(1.2)\\ \hline
MNLI , ALL
      &  89.5(1.9) & 61.9(2.3) & 53.1(1.1)\\

    % & DA & 84.2 & 90.9 & 91 & 28 \\ \midrule
    
    -PAWS
      &82.6(2.7) & 58.2(5.2) & 53.1(1.7)\\
    -QQP
     &  80.1(3.7) & 58.1(5.2) & 51.4(0.6) \\ 
    -SNLI
     &85.4(1.0)  & 61.1(2.2) & 54.3(1.0) \\ 
     
     \hline
     MNLI, PAWS
     & 82.3(1.8) & 59.4(3.9) & 52.8(1.0)\\ \hline    
%MNLI , SNLI + PAWS + QQP, $\gamma=5$
%      & 83.6 & 90.3 &  & & \\
     \bottomrule
\end{tabular}
    \caption{\label{tab:finalnli_more}The NLI experiment results of \bert on HANS three subsets: lexical overlap (HANS-O), constituent (HANS-C) and subsequence (HANS-S) when adding different auxiliary dataset: SNLI, \pawsqqp, \pawswiki, HANS. ALL = SNLI + PAWS + QQP. The numbers in the bracket are the standard deviations of the 5 runs.}
    \end{center}
    }
\end{table*}
